# Supplementary material for: Diffusion Mean Estimation on the Diagonal of Product Manifolds
Source: arXiv:2112.00871 source file (2022-05-24)
Supplement: Supplementary file 1 [file Appendix_A.tex]

\appendix

\section{Appendix A}\label{sec: appendix a}

\begin{proof}[Proof of \reflemma{lemma: Laplace-beltrami on product}]
    This is an elementary fact. Let $(x_1,\dots, x_{nd})$ be local coordinates of $M^n$. The Riemannian metric $g$ on $M^n$ is a block-diagonal matrix with $\text{diag}(g) = (g_1,\dots, g_n)$. Then from the description of the Laplace-Beltrami operator in local coordinates, with $G = \det(g) = \det(g_1) \cdots \det(g_n)$, we see
        \begin{align*}
            \Delta_{M^n} f & = \sum_{i,j = 1}^{nd} \frac{1}{\sqrt{G}}\partiel{x_i} \left( \sqrt{G}g^{ij}\partiel{x_j} f \right)
            \\
            & = \sum_{i,j = 1}^{nd} \frac{1}{\sqrt{\det(g_1)}}\partiel{x_i} \left( \sqrt{\det(g_1)}g^{ij}\partiel{x_j} f \right) + \\
            & \dots + \sum_{i,j = d(n-1)+1}^{nd} \frac{1}{\sqrt{\det(g_n)}}\partiel{x_i} \left( \sqrt{\det(g_n)}g^{ij}\partiel{x_j} f \right)
            \\
            &= \Delta_{M_1}f + \dots + \Delta_{M_n}f,
        \end{align*}
    for any $f \in C^{\infty}(M^n)$.
    \end{proof}

    \begin{proof}[Proof of \reflemma{lemma: Brownian motion on product manifold}]
    Let $\Delta_{O(M^n)}$ be the horizontal lift of $\Delta_{M^n}$ and let $U$ denote the stochastic development of $X$. For any smooth function $\tilde f \colon O(M^n) \rightarrow \R$, we have
        \begin{equation*}
            M^{\tilde f}_t = \tilde f(U_t) - \tilde f(U_0) - \frac{1}{2}\int_0^t \Delta_{O(M^n)}\tilde f(U_s)ds.
        \end{equation*}
    In particular, for any $f \in C^{\infty}(M^n)$ and $\tilde f = f \circ \pi$, with $\pi \colon O(M^n) \rightarrow M^n$ the canonical projection, we have
        \begin{align*}
            M^{\tilde f}_t &= f(X_t) - f(X_0) - \frac{1}{2}\int_0^t \Delta_{M^n}f(X_s)ds
            \\
            &=
            f(X_t) - f(X_0) - \frac{1}{2}\int_0^t \left(\Delta_{M_1}+\dots + \Delta_{M_n}\right)f(X_s)ds.
        \end{align*}
    Define the functions $f_j \in C^{\infty}(M^n)$ by $f_j = g \circ \pi_j$, for any $g \in C^{\infty}(M_j)$, then from the above equation
        \begin{align*}
            M^{f_j}_t &= g(X^j_t) - g(X^j_0) - \frac{1}{2}\int_0^t \Delta_{M_j}g(X^j_s)ds,
        \end{align*}
    hence each $X^j$ is a Brownian motion on $M_j$.
    \end{proof}
