# Supplementary material for: Diffusion Mean Estimation on the Diagonal of Product Manifolds
Source: arXiv:2112.00871 source file (2022-05-24)
Supplement: Supplementary file 3 [file Appendix_C.tex]

\section{Appendix C}

In this section, we consider the Doob's $h$-transform of the sort of conditioning that we are considering. The conditioning is similar to the conditioning in \cite{van2018bayesian}. Throughout, let $p$ denote the transition density of a diffusion process $X$ and $q$ an auxiliary density. Define, for any $t\in [u,T)$, the $h$-function as 
    \begin{equation}
        h(u,X_u) = \int \int \frac{p(u,X_u;t,y)q_{T-t}(y,v)}{\int \int p(0,x_0;t,y)q_{T-t}(y,v) dydv}dydv.
    \end{equation}
Clearly, $h(0,X_0)= 1$ and $h$ defines a local martingale since, for $s<u<t$, by Fubini's theorem
    \begin{align*}
        \E\left[h(u,X_u)|X_s\right] 
        & 
        =
        \int p(s,X_s;u,x) h(u,x) dx 
        \\
        &
        = 
        \int p(s,X_s;u,x) \int \int \frac{p(u,x;t,y)q_{T-t}(y,v)}{\int \int p(0,x_0;t,y)q_{T-t}(y,v) dydv}dydv dx
        \\
        &
        =
        \int \int  \frac{\int p(s,X_s;u,x)p(u,x;t,y)dx }{\int \int p(0,x_0;t,y)q_{T-t}(y,v) dydv}q_{T-t}(y,v)dydv 
        \\
        &
        =\int \int  \frac{ p(s,X_s;t,y)q_{T-t}(y,v) }{\int \int p(0,x_0;t,y)q_{T-t}(y,v) dydv}dydv.
    \end{align*}
We thus have a new probability measure $\Pb^h$ defined on $\cF_{T-}$ and we obtain a conditioning, since for any bounded measurable $f$
    \begin{align*}
        \E^{\Pb^h}\left[f(X_u)\right] 
        &
        =
        \int f(x) p(s,X_s;u,x) \int \int \frac{p(u,x;t,y)q_{T-t}(y,v)}{\int \int p(0,x_0;t,y)q_{T-t}(y,v) dydv}dydv dx
        \\
        &
        = 
        \int \int \left(\int f(x) \frac{p(0,x_0;u,x)p(u,x;t,y)}{p(0,x_0;t,y)}dx \right) \xi_t(y,v) dy dv
        \\
        &
        =
        \int \int \E\left[f(X_u)|X_t = y\right] \xi_t(y,v) dy dv,
    \end{align*}
where 
    \begin{equation}
        \xi_t(y,v) = \frac{p(0,x_0;t,y) q_{T-t}(y,v)}{\int p(0,x_0;t,y)q_{T-t}(y,v) dydv}.
    \end{equation}
